# Supplementary material for: Wrench-Based Bayesian Pose Estimation via Matrix Fisher-Gaussian Inference
Source: arXiv:2607.07306 source file (2026-12-01)
Supplement: Supplementary file 1 [file supplementary_refmap.tex]

% Numbers and destinations from the companion document.
\makeatletter
\def\CrossDocumentSMMapVersion{20261124}
\providecommand{\SMPDFFile}{SM.pdf}
\expandafter\def\csname CrossDocumentSMnumber@alg:opt-newton\endcsname{S7.1}
\expandafter\def\csname CrossDocumentSMname@alg:opt-newton\endcsname{Algorithm}
\expandafter\def\csname CrossDocumentSManchor@alg:opt-newton\endcsname{algorithm.comparison.S7.1}
\expandafter\def\csname CrossDocumentSMnumber@app:opt-distribution-errors\endcsname{S7.4}
\expandafter\def\csname CrossDocumentSMname@app:opt-distribution-errors\endcsname{Section}
\expandafter\def\csname CrossDocumentSManchor@app:opt-distribution-errors\endcsname{subsection.7.4}
\expandafter\def\csname CrossDocumentSMnumber@app:opt-evidence\endcsname{S7}
\expandafter\def\csname CrossDocumentSMname@app:opt-evidence\endcsname{Section}
\expandafter\def\csname CrossDocumentSManchor@app:opt-evidence\endcsname{section.7}
\expandafter\def\csname CrossDocumentSMnumber@app:opt-newton\endcsname{S7.1}
\expandafter\def\csname CrossDocumentSMname@app:opt-newton\endcsname{Section}
\expandafter\def\csname CrossDocumentSManchor@app:opt-newton\endcsname{subsection.7.1}
\expandafter\def\csname CrossDocumentSMnumber@app:opt-reconstruction-cost\endcsname{S7.2}
\expandafter\def\csname CrossDocumentSMname@app:opt-reconstruction-cost\endcsname{Section}
\expandafter\def\csname CrossDocumentSManchor@app:opt-reconstruction-cost\endcsname{subsection.7.2}
\expandafter\def\csname CrossDocumentSMnumber@supp:posterior-extensions\endcsname{S6}
\expandafter\def\csname CrossDocumentSMname@supp:posterior-extensions\endcsname{Section}
\expandafter\def\csname CrossDocumentSManchor@supp:posterior-extensions\endcsname{section.6}
\expandafter\def\csname CrossDocumentSMnumber@supp:s1-geometry\endcsname{S1.1}
\expandafter\def\csname CrossDocumentSMname@supp:s1-geometry\endcsname{Section}
\expandafter\def\csname CrossDocumentSManchor@supp:s1-geometry\endcsname{subsection.1.1}
\expandafter\def\csname CrossDocumentSMnumber@supp:s1-potential\endcsname{S1.2}
\expandafter\def\csname CrossDocumentSMname@supp:s1-potential\endcsname{Section}
\expandafter\def\csname CrossDocumentSManchor@supp:s1-potential\endcsname{subsection.1.2}
\expandafter\def\csname CrossDocumentSMnumber@supp:s2-nested-results\endcsname{S2.2}
\expandafter\def\csname CrossDocumentSMname@supp:s2-nested-results\endcsname{Section}
\expandafter\def\csname CrossDocumentSManchor@supp:s2-nested-results\endcsname{subsection.2.2}
\expandafter\def\csname CrossDocumentSMnumber@supp:s2-selection\endcsname{S2.1}
\expandafter\def\csname CrossDocumentSMname@supp:s2-selection\endcsname{Section}
\expandafter\def\csname CrossDocumentSManchor@supp:s2-selection\endcsname{subsection.2.1}
\expandafter\def\csname CrossDocumentSMnumber@supp:s3-cost\endcsname{S3.1}
\expandafter\def\csname CrossDocumentSMname@supp:s3-cost\endcsname{Section}
\expandafter\def\csname CrossDocumentSManchor@supp:s3-cost\endcsname{subsection.3.1}
\expandafter\def\csname CrossDocumentSMnumber@supp:s3-probability-errors\endcsname{S3.2}
\expandafter\def\csname CrossDocumentSMname@supp:s3-probability-errors\endcsname{Section}
\expandafter\def\csname CrossDocumentSManchor@supp:s3-probability-errors\endcsname{subsection.3.2}
\expandafter\def\csname CrossDocumentSMnumber@supp:s3-reference-checks\endcsname{S3.3}
\expandafter\def\csname CrossDocumentSMname@supp:s3-reference-checks\endcsname{Section}
\expandafter\def\csname CrossDocumentSManchor@supp:s3-reference-checks\endcsname{subsection.3.3}
\expandafter\def\csname CrossDocumentSMnumber@supp:s3-sampling-diagnostics\endcsname{S3.4}
\expandafter\def\csname CrossDocumentSMname@supp:s3-sampling-diagnostics\endcsname{Section}
\expandafter\def\csname CrossDocumentSManchor@supp:s3-sampling-diagnostics\endcsname{subsection.3.4}
\expandafter\def\csname CrossDocumentSMnumber@supp:s4:apparatus\endcsname{S5.1}
\expandafter\def\csname CrossDocumentSMname@supp:s4:apparatus\endcsname{Section}
\expandafter\def\csname CrossDocumentSManchor@supp:s4:apparatus\endcsname{subsection.5.1}
\expandafter\def\csname CrossDocumentSMnumber@supp:s4:physical-validation\endcsname{S5}
\expandafter\def\csname CrossDocumentSMname@supp:s4:physical-validation\endcsname{Section}
\expandafter\def\csname CrossDocumentSManchor@supp:s4:physical-validation\endcsname{section.5}
\expandafter\def\csname CrossDocumentSMnumber@supp:s4:results\endcsname{S5.2}
\expandafter\def\csname CrossDocumentSMname@supp:s4:results\endcsname{Section}
\expandafter\def\csname CrossDocumentSManchor@supp:s4:results\endcsname{subsection.5.2}
\expandafter\def\csname CrossDocumentSMnumber@supp:sec:geometry-contact\endcsname{S1}
\expandafter\def\csname CrossDocumentSMname@supp:sec:geometry-contact\endcsname{Section}
\expandafter\def\csname CrossDocumentSManchor@supp:sec:geometry-contact\endcsname{section.1}
\expandafter\def\csname CrossDocumentSMnumber@supp:shape-clouds\endcsname{S4}
\expandafter\def\csname CrossDocumentSMname@supp:shape-clouds\endcsname{Section}
\expandafter\def\csname CrossDocumentSManchor@supp:shape-clouds\endcsname{section.4}
\expandafter\def\csname CrossDocumentSMnumber@supp:shape-geometry-controls\endcsname{S4.2}
\expandafter\def\csname CrossDocumentSMname@supp:shape-geometry-controls\endcsname{Section}
\expandafter\def\csname CrossDocumentSManchor@supp:shape-geometry-controls\endcsname{subsection.4.2}
\expandafter\def\csname CrossDocumentSMnumber@supp:tab:baseline\endcsname{S1}
\expandafter\def\csname CrossDocumentSMname@supp:tab:baseline\endcsname{Table}
\expandafter\def\csname CrossDocumentSManchor@supp:tab:baseline\endcsname{table.caption.1}
\expandafter\def\csname CrossDocumentSMnumber@supp:tab:k-rotation\endcsname{S3}
\expandafter\def\csname CrossDocumentSMname@supp:tab:k-rotation\endcsname{Table}
\expandafter\def\csname CrossDocumentSManchor@supp:tab:k-rotation\endcsname{table.caption.3}
\expandafter\def\csname CrossDocumentSMnumber@supp:tab:k-translation\endcsname{S4}
\expandafter\def\csname CrossDocumentSMname@supp:tab:k-translation\endcsname{Table}
\expandafter\def\csname CrossDocumentSManchor@supp:tab:k-translation\endcsname{table.caption.4}
\expandafter\def\csname CrossDocumentSMnumber@supp:tab:runtime-repeats\endcsname{S9}
\expandafter\def\csname CrossDocumentSMname@supp:tab:runtime-repeats\endcsname{Table}
\expandafter\def\csname CrossDocumentSManchor@supp:tab:runtime-repeats\endcsname{table.caption.12}
\newcommand{\SMNumber}[1]{%
  \ifcsname CrossDocumentSMnumber@#1\endcsname%
    \csname CrossDocumentSMnumber@#1\endcsname%
  \else%
    \PackageError{CrossDocument}{Missing SM reference: #1}{Use the paired reference map from this release.}%
    \textbf{??}%
  \fi}
% arXiv builds use versioned HTTPS links. The editable pair uses sibling PDFs.
\ifdefined\ArxivProjectDirectory\else
  \InputIfFileExists{arxiv-public-links.cfg}{}{}%
\fi
\newcommand{\CrossDocumentSMLink}[2]{%
  \ifcsname CrossDocumentSManchor@#1\endcsname%
    \ifdefined\ArxivCrossLink%
      \ArxivCrossLink{SM}{\csname CrossDocumentSManchor@#1\endcsname}{#2}%
    \else%
      \hyper@linkfile{#2}{\SMPDFFile}{\csname CrossDocumentSManchor@#1\endcsname}%
    \fi%
  \else%
    \PackageError{CrossDocument}{Missing SM PDF target: #1}{Use the paired reference map from this release.}%
  \fi}
\DeclareRobustCommand{\SMref}[1]{\CrossDocumentSMLink{#1}{\SMNumber{#1}}}
\DeclareRobustCommand{\SMeqref}[1]{\textup{\CrossDocumentSMLink{#1}{(\SMNumber{#1})}}}
\DeclareRobustCommand{\SMCref}[1]{\CrossDocumentSMLink{#1}{\csname CrossDocumentSMname@#1\endcsname~\SMNumber{#1}}}
\DeclareRobustCommand{\SMcref}[1]{\SMCref{#1}}
\makeatother
